# Supplementary material for: Colloidal hydrodynamic interactions in viscoelastic fluids
Source: arXiv:2508.11948 ancillary file (2025-08-19)
Supplement: Supplementary file 1 [file Supplementary_Information.pdf]

# Supplementary Information for:
Colloidal hydrodynamic interactions in viscoelastic fluids

Dae Yeon Kim[1,*], Sachit G. Nagella[1,*], Saksham Malik[1], Nayeon Park[2], Jaewook Nam[2,3], Eric S.G. Shaqfeh[1,4], Sho C. Takatori[1,†]

[1]Department of Chemical Engineering, Stanford University, CA, USA
[2]Department of Chemical and Biological Engineering, Seoul National University, Seoul, Korea
[3]Institute of Chemical Processes, Seoul National University, Seoul, Korea
[4]Department of Mechanical Engineering, Stanford University, CA, USA

[*]These authors contributed equally to this work.
[†]Corresponding author: stakatori@stanford.edu

August 19, 2025

## 1 Experimental setup

### 1.1 Mechanical Characterization of Wormlike Micellar Solutions

The structural length scales and characteristic relaxation times of the wormlike micellar (WLM) solution used in the experiments were characterized via rheological measurements. All rheological tests were performed using a rotational rheometer (DHR-3, TA Instruments) equipped with a 40 mm parallel-plate geometry at 20 °C. To prevent evaporation during measurements, an antievaporation solvent trap was employed. We first measured the viscosity of the wormlike micellar solutions under simple shear flow. The resulting zero-shear viscosities were determined to be 4.17 mPa·s for the 0.25 wt% in water sample, 1500 mPa·s for the 0.25 wt% in 0.5 M NaCl sample, and 127 mPa·s for the 0.125 wt% in 0.5 M NaCl sample (Fig. S1A).

The characteristic time scales of mesoscopic wormlike micelles can be inferred from their viscoelastic behavior. Under small-amplitude oscillatory shear, wormlike micelle solutions are known to exhibit Maxwell behavior, characterized by a single dominant relaxation time (Fig. S1B). The relaxation time, $\lambda$, was determined by fitting the storage ($G'$) and loss ($G''$) moduli to a single-mode Maxwell element:

$$G'(\omega) = \frac{G_0\omega^2\lambda^2}{1+\omega^2\lambda^2}, \tag{1}$$

$$G''(\omega) = \frac{G_0\omega\lambda}{1+\omega^2\lambda^2}, \tag{2}$$

where $G_0$ is the plateau value of the elastic modulus and $\omega$ is the angular frequency. We obtained the relaxation time from the the crossover frequency, $\lambda = \omega_c^{-1}$, where $G'(\omega_c) = G''(\omega_c)$. The relaxation times were approximately 250 ms, 670 ms, and 310 ms for the 0.25 wt% in water, 0.25 wt% in 0.5 M NaCl, and 0.125 wt% in 0.5 M NaCl solutions, respectively. All small-amplitude oscillatory shear tests were conducted at a fixed shear strain of 5%, which was confirmed to lie within the linear viscoelastic regime based on amplitude sweep measurements.

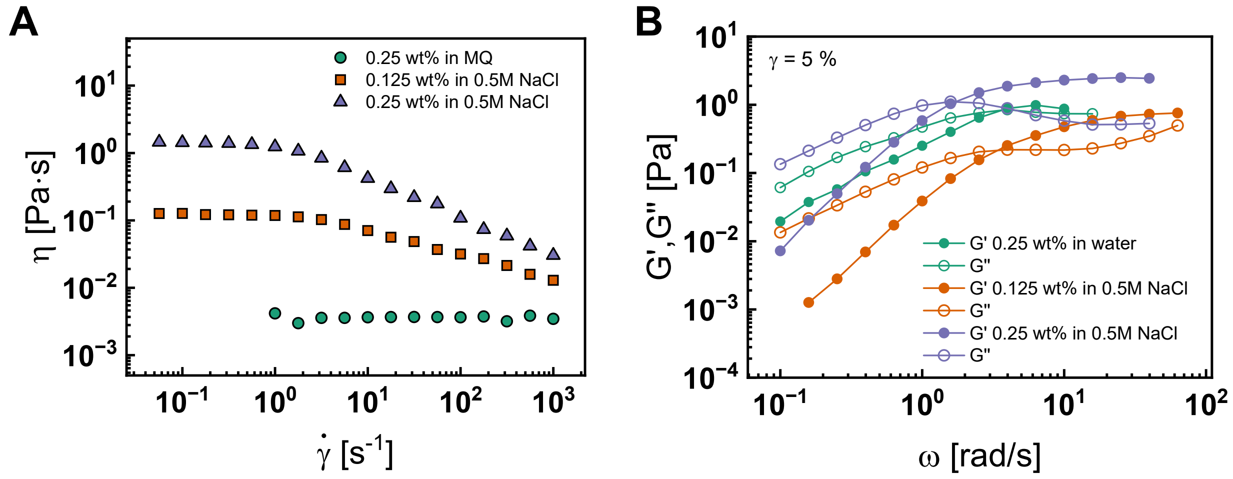


Figure S1: Rheological characterization of wormlike micellar solutions. (A) Flow curves obtained from steady shear experiments, showing the zero-shear viscosity and shear-thinning behavior for different WLM samples. (B) Small-amplitude oscillatory shear results measured at 5% strain, confirming the linear viscoelastic regime and allowing extraction of the characteristic relaxation time from the crossover point of $G'$ and $G''$.

The mesh size ($\xi_M$) of the entangled WLM network is estimated using the plateau modulus [1, 2]

$$\xi_M = \left(\frac{k_B T}{G_0}\right)^{1/3}, \tag{3}$$

where $k_B$ is the Boltzmann constant and $T$ is the absolute temperature. The resulting values of $\xi_M$ were approximately 160 nm, 120 nm, and 200 nm for the 0.25 wt% in water, 0.25 wt% in 0.5 M NaCl, and 0.125 wt% in 0.5 M NaCl samples, respectively.

The average micelle contour length ($L_c$) of the WLM solution was estimated based on established scaling relations involving the $G_0$, the local minimum of the loss modulus ($G''_{\text{min}}$), and the entanglement length [1, 2]. The entanglement length, defined as the average distance between successive entanglement points along the micelle chain, was obtained through its scaling relation with $G_0$ and the persistence length of micelle ($l_p$) [2, 3, 4]. Using reported values of the persistence length ($l_p \sim 25$ nm) in similar WLM system [5, 4], we estimated $L_c$ for our samples. The values of $L_c$ were approximately 0.72 µm, 3.5 µm, and 1.1 µm for the 0.25 wt% in water, 0.25 wt% in 0.5 M NaCl, and 0.125 wt% in 0.5 M NaCl samples, respectively.

We compared the relaxation times of WLM solutions obtained from the transient start-up in the probe's angular displacement with those measured using a conventional macrorheometer. We included data for all three wormlike micellar (WLM) samples, including the 0.125 wt% in 0.5M NaCl solution that was not shown in the main text (see orange box plot in Fig. S2). The median relaxation time of 0.125 wt% in 0.5M NaCl solution was 303 ms, agreeing with those obtained from the bulk rheological measurements. All samples exhibited excellent agreement between the two methods.

## 1.2 Colloidal particles with hemispherical fluorescent coating

Amino-functionalized poly(methyl methacrylate) (PMMA) particles (5% w/v, Abvigen Inc.) were hemispherically labeled with fluorescent dye using the gel trapping technique [6]. First, a 2 wt % gellan gum aqueous solution (Phytagel, Sigma-Aldrich, USA) was poured into a Petri dish and n-Decane (Sigma-Aldrich, USA) was added to create an oil-water interface. A solution, containing

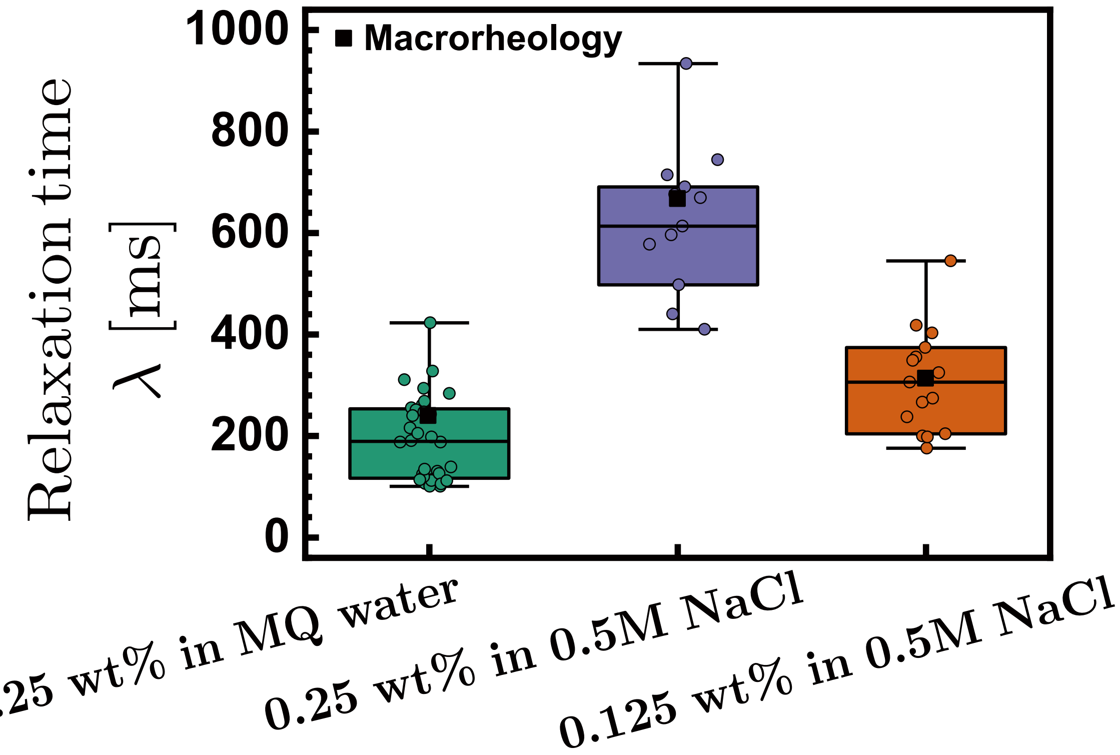


Figure S2: Expanded version of Fig. 2C in the main text comparing measurements of relaxation times of wormlike micellar solutions from optical tweezer experiments and conventional rheometry. From left to right, the median values of the relaxation times are 189, 614, and 303 ms. Corresponding relaxation times obtained from the crossover frequency in small-amplitude oscillatory shear rheometry are 250, 670, and 310 ms (black squares)

washed amino PMMA particles mixed with isopropyl alcohol (IPA), was carefully introduced to the interface using a micropipette, thereby positioning the particles at the interface. The system was then cooled at room temperature for approximately one hour, allowing gelation of the gellan gum solution beneath the interface. After n-Decane was removed, a poly(dimethylsiloxane) (PDMS) silicone elastomer (Sylgard 184, Dow, USA) was poured over the gelled solution and left to cure for two days. Upon curing, the PDMS was carefully peeled off from the gellan gum, capturing the PMMA particles that were partially embedded on one side. To fluorescently label the particles, the amine groups on the surface of the particle reacted with Alexa Fluor 647 NHS Ester (Invitrogen, USA) by NHS ester-amine coupling. The fluorescent particles were then collected using water-soluble polyvinyl alcohol (PVA) tape dissolved in Milli-Q water, and centrifuged to isolate the particles. The isolated particles were washed multiple times with warm Milli-Q water and subsequently diluted for experimental use.

### 1.3 Observation setup

All measurements described in this study were conducted using the setup schematically illustrated in Fig. 1A. The observation cell was assembled on a glass coverslip (170±5 µm thickness, Marienfeld) using a PDMS chamber with a 6 mm diameter hole and a height of 5 mm, which served as the side wall. Two hemispherical fluorescent particles were trapped at a fixed center-to-center separation. They were positioned far from the chamber walls, the air–water interface, and the bottom surface to avoid confinement effects. Experiments were conducted under dilute conditions, such that the

influence of other particles outside the trapped pair could be neglected. Subsequently, as shown in Fig. 1B, one of the particles was driven along a circular trajectory at constant speed.

# 2 Continuum Simulations

## 2.1 Governing Equations

To model the experimental setup, we consider two spheres of radius $a$ placed within a spherical computational domain of radius $R = 25a$. The probe sphere is located at the center of the domain, while the outer sphere is positioned at a distance $r$ from the center of the probe sphere.

The surrounding fluid is governed by the conservation laws for mass and momentum, written in non-dimensional form as:

$$\frac{\partial u_i}{\partial x_i} = 0, \tag{4}$$

$$Re\left(\frac{\partial u_i}{\partial t} + u_j \frac{\partial u_i}{\partial x_j}\right) = \frac{\partial \sigma_{ij}}{\partial x_j}, \tag{5}$$

where $u_i$ is the fluid velocity and $\sigma_{ij}$ is the total fluid stress. The equations are nondimensionalized using the particle radius $a$ as the characteristic length scale, the inverse of the imposed angular velocity $\dot{\theta}^{-1}$ as the time scale, and $a\dot{\theta}$ as the velocity scale. Stress is scaled by $\eta_0 a\dot{\theta}$, where $\eta_0$ is the total viscosity of the suspending fluid. The Reynolds number is defined as $Re = \rho a^2\dot{\theta}/\eta_0$, where $\rho$ is the fluid density. The total stress in the system, $\sigma_{ij}$, can be decomposed into a Newtonian contribution and a polymeric contribution as follows -

$$\sigma_{ij} = -p\delta_{ij} + \beta\left(\frac{\partial u_i}{\partial x_j} + \frac{\partial u_j}{\partial x_i}\right) + \sigma^p_{ij}, \tag{6}$$

where $p$ is the pressure of the fluid, and $\beta = \eta_s/\eta_0 = \eta_s/(\eta_s + \eta_p)$ is the ratio of solvent viscosity $\eta_s$ to the total viscosity $\eta_0$ of the suspending fluid, where $\eta_p$ is the polymeric contribution, $\sigma^p_{ij}$ is the polymeric contribution to the total stress.

To close these equations, we use a constitutive model for the polymeric stress, $\sigma^p_{ij}$. In the simulations described below, the Oldroyd-B constitutive model is used, modeling the polymeric solution as a dilute suspension of Hookean dumbbells. Coarse-grained elastic dumbbells are represented by the polymer conformation tensor, $c_{ij} = \langle R_i R_j \rangle$, where $R_i$ is the end-to-end vector of the polymer dumbbell. It is made dimensionless using the radius of gyration of the dumbbell. The upper-convected Oldroyd-B model describes the evolution of $c_{ij}$,

$$\frac{\partial c_{ij}}{\partial t} + u_k \frac{\partial c_{ij}}{\partial x_k} - c_{ik}\frac{\partial u_j}{\partial x_k} - c_{kj}\frac{\partial u_i}{\partial x_k} = -\frac{1}{Wi}\left(c_{ij} - \delta_{ij}\right), \tag{7}$$

The Weissenberg number is defined as $Wi = \lambda\dot{\gamma}_0 = \lambda U/(r - 2a)$, where $\lambda$ is the polymer relaxation time and $\dot{\gamma}_0$ is the characteristic strain-rate in the gap between the spheres. We choose to scale the strain-rate $\dot{\gamma}_0 = U/(r - 2a)$, where $U$ is the translational velocity of the outer sphere and $r - 2a$ is the surface-to-surface distance between the spheres. From the Oldroyd-B model, we determine the polymer contribution to the total fluid stress,

$$\sigma^P_{ij} = \frac{1-\beta}{Wi}\left(c_{ij} - \delta_{ij}\right). \tag{8}$$

## 2.2 Numerical Setup

Direct numerical solutions were computed using a parallelized, fully three-dimensional, unstructured finite-volume, incompressible flow solver. A boundary-fitted computational domain conforming to the geometry of the spheres was used to simulate particles in either a Newtonian or viscoelastic fluid. The computational domain was a sphere of radius $R = 25a$. An unstructured tetrahedral mesh was employed, with finer elements of size $a/12.5$ near the particle surfaces and coarser resolution near the outer boundaries. A schematic of this system is shown in Fig. S3

The simulations were conducted in the reference frame of the outer sphere, which is held stationary. At $t = 0$, all fluid elements and the probe sphere are initialized with a translational velocity equal in magnitude and opposite in direction to that of the outer sphere $u_i = -\epsilon_{ijk}\,\dot{\theta}_j\,x_k$. This initialization ensures the correct relative motion in the rotating frame. To simulate the stopping of the outer sphere, the same angular velocity as above is injected in the opposite direction into each fluid element.

A no-slip boundary condition is imposed on the fluid domain boundary as well as the surface of the outer sphere in the reference frame of the outer sphere. The probe sphere is constrained to be torque-free at all times with a no-slip boundary condition on the surface. At each time step, Broyden's method is used to iteratively solve for the instantaneous angular velocity of the probe [7]. The mesh and time step sizes were chosen based on convergence tests, ensuring that further refinement resulted in less than 5% changes to the computed dimensionless angular velocities.

Extensive details on the solver, including validation cases and comparison to experiments, can be found in prior studies [8, 9, 10, 11].

## 2.3 Validation of results

Before simulating the motion of the spheres in a viscoelastic fluid, it was important to validate the results from the direct numerical solutions by comparing them to previous results obtained by Kim et al [12]. Simulations were first performed in a Newtonian fluid and compared with theoretical results, Stokesian dynamics and experimental results (Fig. S4). The results show that the steady angular velocities of the stationary probe agree with those from experiments, Stokesian dynamics calculations, and analytical predictions at various separation distances.

## 2.4 Viscoelastic simulation results and discussion

Viscoelastic fluid simulations were performed using the Oldroyd-B model using different values of $\beta$, the viscosity partition coefficient, which decreases as the polymer viscosity contribution increases. Based on rheology, a $\beta$ value of 0.001 is obtained. However, we used a range of $\beta$ values with the same total viscosity at a separation of $r = 4.4a$ (corresponding to $Wi = 1.17$) to capture the effects of changing the polymer-solvent viscosity ratio in a Oldroyd-B fluid on the rotation-translation hydrodynamic coupling. For all different ratios of solvent-polymer viscosities in the simulation for viscoelastic fluids, the inner probe reaches close to the Newtonian steady state on the order of the momentum relaxation timescale, as shown in Fig. S5. However, there appears to be some transience as the angular velocity of the probe oscillates about the Newtonian value on the order of the relaxation timescale of the fluid. It is also worth noting that after stopping the moving particle (at $1.5\lambda$), the probe reverses its direction, although very slightly, as indicated by the negative angular velocities in that period. The magnitude of this reversal increases with a decrease in $\beta$ while a negative angular velocity during reversal is not observed at $\beta = 0.7$. To further explore this effect, we lowered $\beta$ more, and the outer particle is moved until the angular velocity of the probe reaches a steady state, as shown in Fig. S6. Viscoelastic simulations with $\beta$ values of 0.1

and 0.01 suggest that the angular velocity of the inner probe reaches a steady state in about 4-6 polymer relaxation times, with a negative angular velocity in the reversal period. It is important to note that the steady state values of the probe angular velocity are 10-20% higher than the values obtained in the simulation for a Newtonian fluid. The case with $\beta = 0.01$ had oscillatory transient behavior with a much higher peak suggesting there are numerical instabilities in the simulation of an Oldroyd-B fluid with a dominant polymer viscosity, even though the steady state is very similar.

To explore the differences in the transient behavior from analytical theory, we decided to run simulations at the same $\beta$ values but at a lower $Wi = 1.17E - 3$. Both cases with $\beta$ values of 0.1 and 0.01 achieve the same steady state as the Newtonian simulation at this low Wi, as shown in Fig. S7. This steady state is similar to theoretical predictions in the main text. Comparing this result to the simulations at the experimental Wi, we see that the climb to a different steady state angular velocity is a finite Wi effect for a continuum fluid (Fig. S8).

Similar simulations were performed at different separation distances corresponding to different Wi for a fixed $\beta$ value of 0.1 as no numerical instabilities were observed at that value. The trace of the conformation tensor, as plotted in Fig. S11, for a separation distance of $r = 2.8a$ (corresponding to $Wi = 3.5$), shows that the normal stress around the sphere grows over several polymer relaxation times until it reaches a steady state in 6-8 polymer relaxation times. This normal stress is concentrated around the 2 spheres with a wake that develops over time.

The angular velocity of the probe achieves a negative velocity during the reversal period, which lasts about 1-2 polymer relaxation times before the angular velocity goes back to zero, which is in contrast to the experiment, where the reversal lasts several relaxation times, or several seconds. The extent of reversal in angular displacement increases when the fluid is wound more around the moving sphere, as shown in Fig. S9. This extent of reversal increases as the number of windings increases to 1 and is then constant. Moreover, the time it takes to undergo one winding here is similar to the time it takes for the probe angular velocity to reach a steady state value. It is important to note that the magnitudes of angular displacement here are much smaller compared to what is observed in the case of the wormlike micelles, but are similar to the ones seen in other polymeric fluids such as PEO, as can be seen in Fig. 4. The plots depicting trace of the conformation tensor in Fig. S11 show that the normal stress relaxes in the opposite direction during this reversal phase.

Moreover, during the reversal phase, the forces on each of the sphere can be calculated by integrating the traction over their surfaces, as shown in Fig. S10. Both the spheres experience an attractive force in the x-direction (separation direction) similar to what is observed in the experiment and Stokesian dynamics simulations in the main text.

# 3 Macrorheology: Creep and Recovery Tests

Macroscopic creep and recovery experiments were conducted using a stress-controlled rheometer (DHR-3, TA Instrument) with a 40 mm parallel plate geometry. A fixed gap of 1000 µm was used, and all tests were performed at 20 °C. For each sample, we applied a constant shear stress for 20 s (creep phase), then set the stress to zero and measured the geometry's displacement for 60 s (recovery phase). Three different suspending fluids were tested: (1) a Newtonian glycerol solution, (2) a semi-dilute polyethylene oxide (PEO) solution (5,000 kg/mol, 0.5 wt%), and (3) a wormlike micelle (WLM) solution (Fig. S12).

For the WLM samples, we applied shear stresses of 1, 20, 100, 200, and 400 Pa, covering a wide range that bracketed and exceeded the estimated stress scale in the optical tweezer experiments (1–10 Pa). Reversal during recovery was only observed in WLMs when high stress levels ($> 20$ Pa)

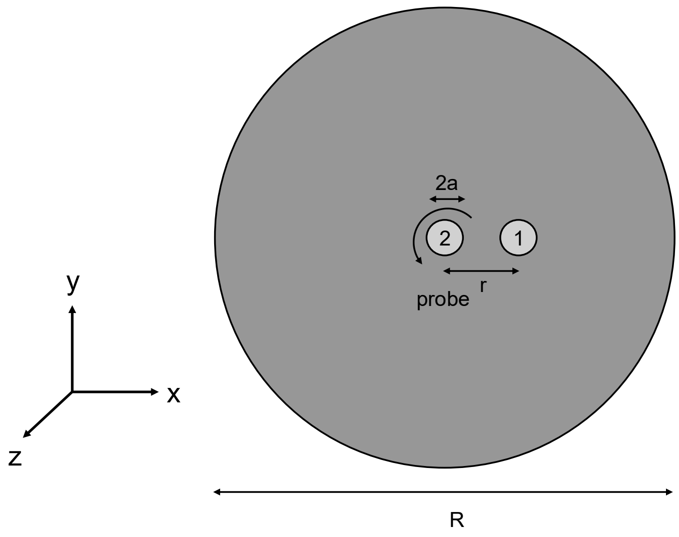


Figure S3: Schematic of the fluid domain used in the direct numerical simulations with 2 spheres separated by some distance,r in the x-direction.

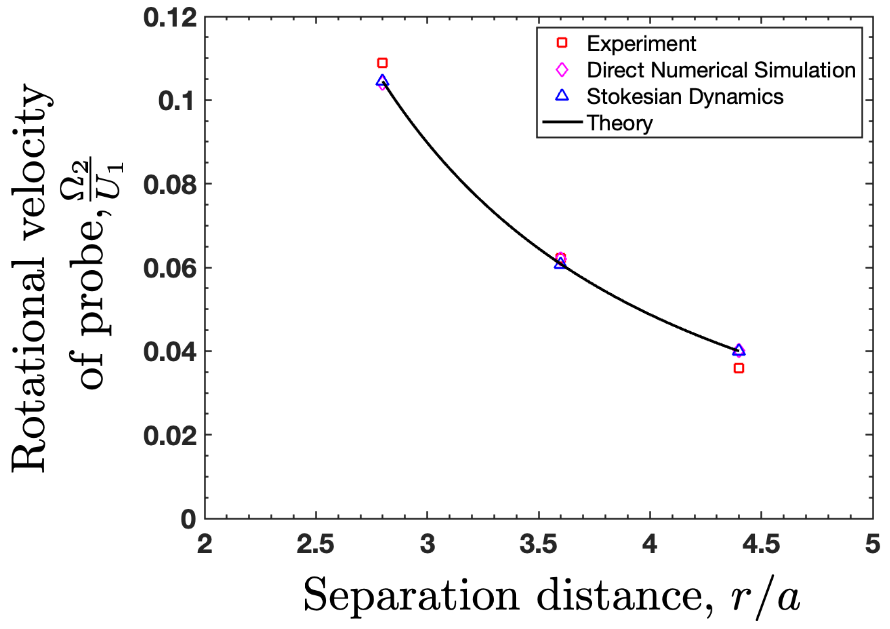


Figure S4: Steady states of the dimensionless Angular velocity for different pairs of separation in a Newtonian fluid.

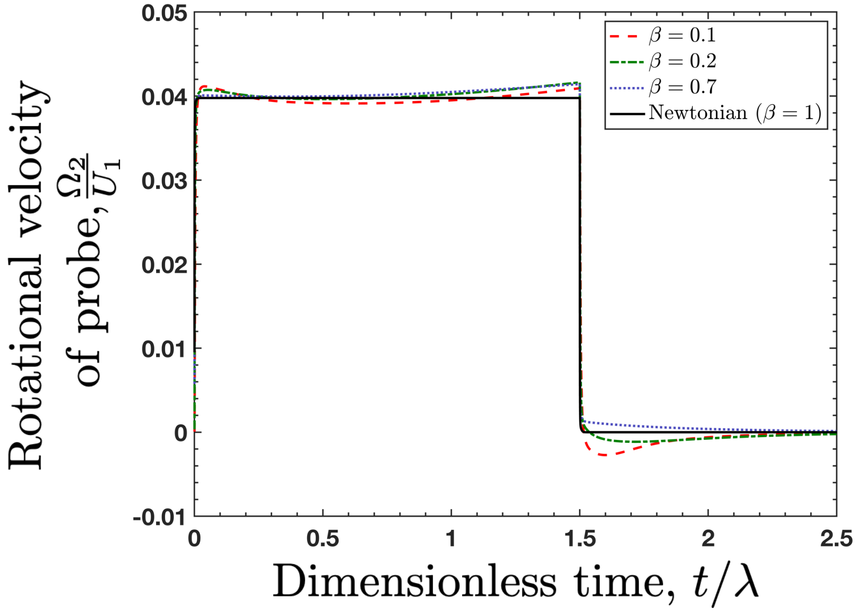


Figure S5: Development of the induced angular velocity of the probe with time normalized by polymer relaxation time for different values of $\beta$ for an Oldroyd-B fluid with Wi=1.17.

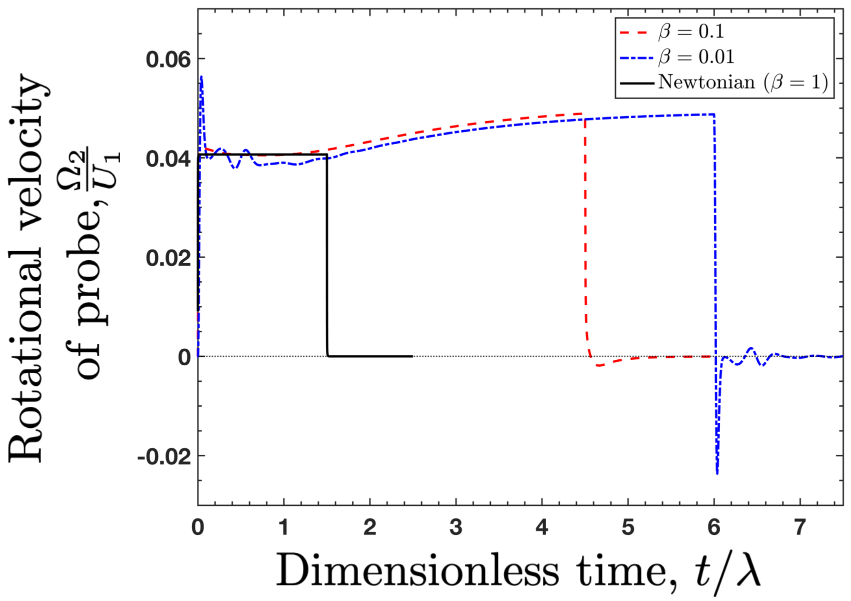


Figure S6: Development of the induced angular velocity of the probe with time normalized by polymer relaxation time for different values of $\beta$ for an Oldroyd-B fluid with Wi number of 1.17, demonstrating that the angular velocity of the probe grows to reach a higher steady state than a Newtonian fluid.

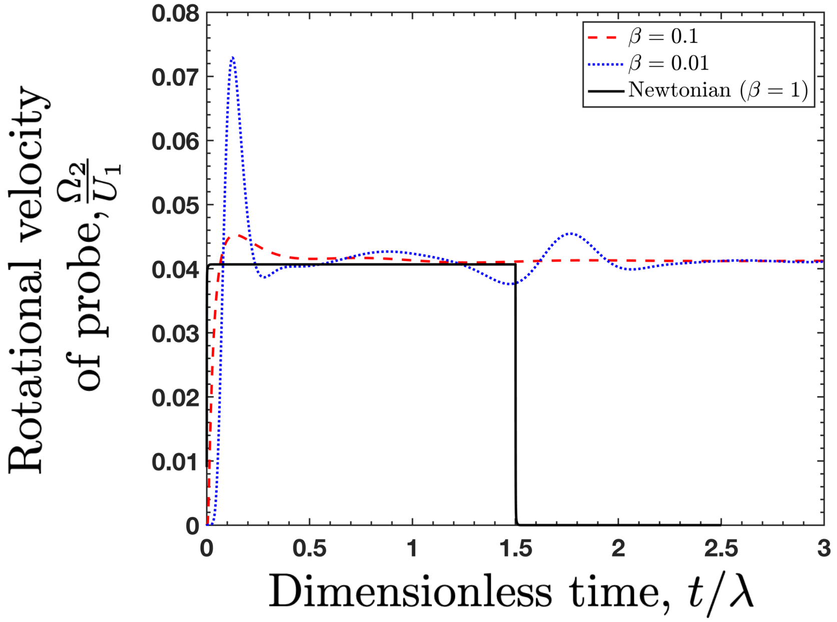


Figure S7: Development of the induced angular velocity of the probe with time normalized by polymer relaxation time for different values of $\beta$ for an Oldroyd-B fluid at Wi=1.17E-3, demonstrating that the steady angular velocity of the probe is similar to a Newtonian fluid.

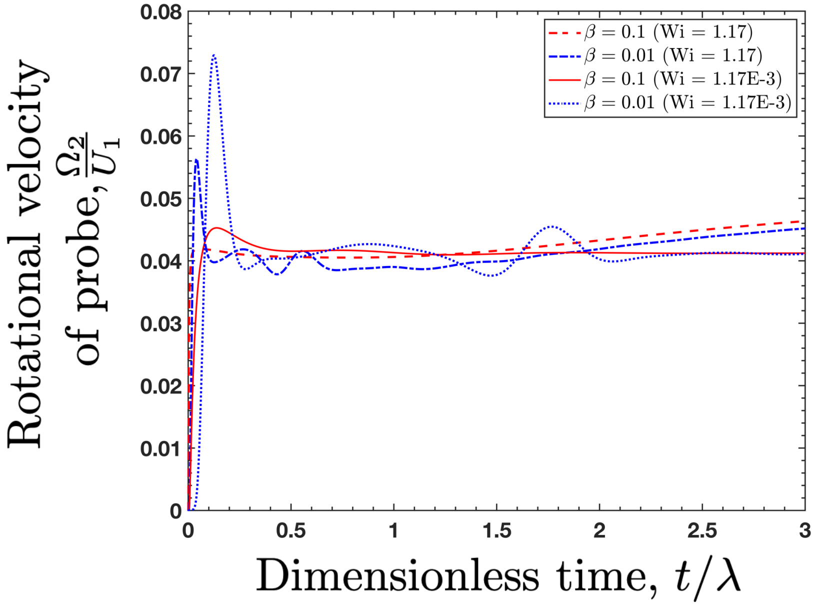


Figure S8: Comparison between the development of the induced angular velocity of the probe for different values of $\beta$ for an Oldroyd B fluid at low Wi number (1.17E-3) and high Wi number (1.17), demonstrating that the steady state angular velocity of the probe is similar to a Newtonian fluid for low Wi suggesting that the climb to a different steady state is a finite Wi number effect.

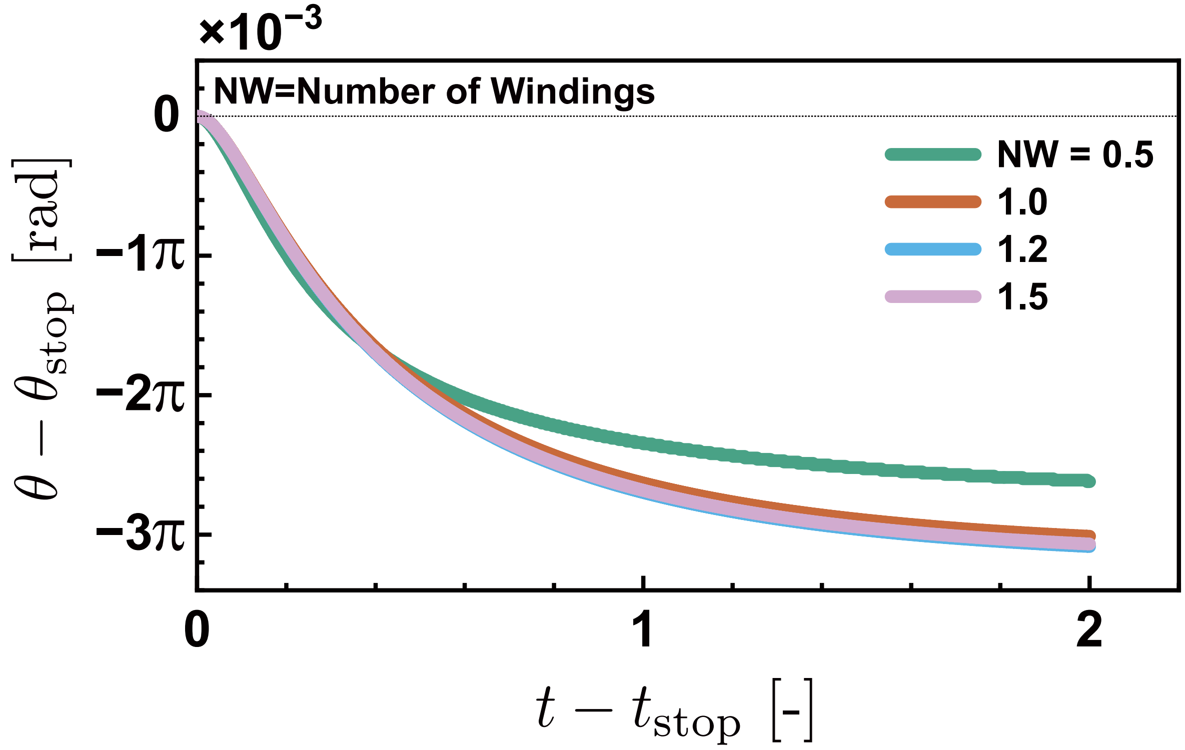


Figure S9: Dependence of angular displacement reversal on the number of windings around the moving sphere for a separation of $r = 2.8a$ corresponding to $Wi = 3.5$ with $\beta = 0.1$. Increasing the number of windings around the moving particle enhances the reversal in probe rotation after flow cessation and the reversal gradually saturates.

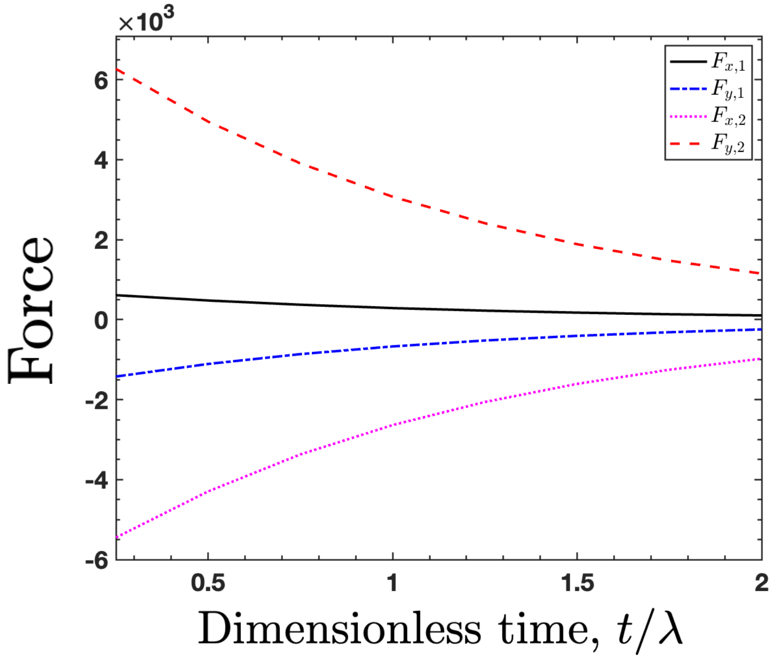


Figure S10: The net force on the probe (sphere 2) and the outer particle (sphere 1) as a function of time post the stopping of the outer sphere shows an attractive force between the 2 spheres for a separation of $r = 2.8a$ corresponding to $Wi = 3.5$ with $\beta = 0.1$.

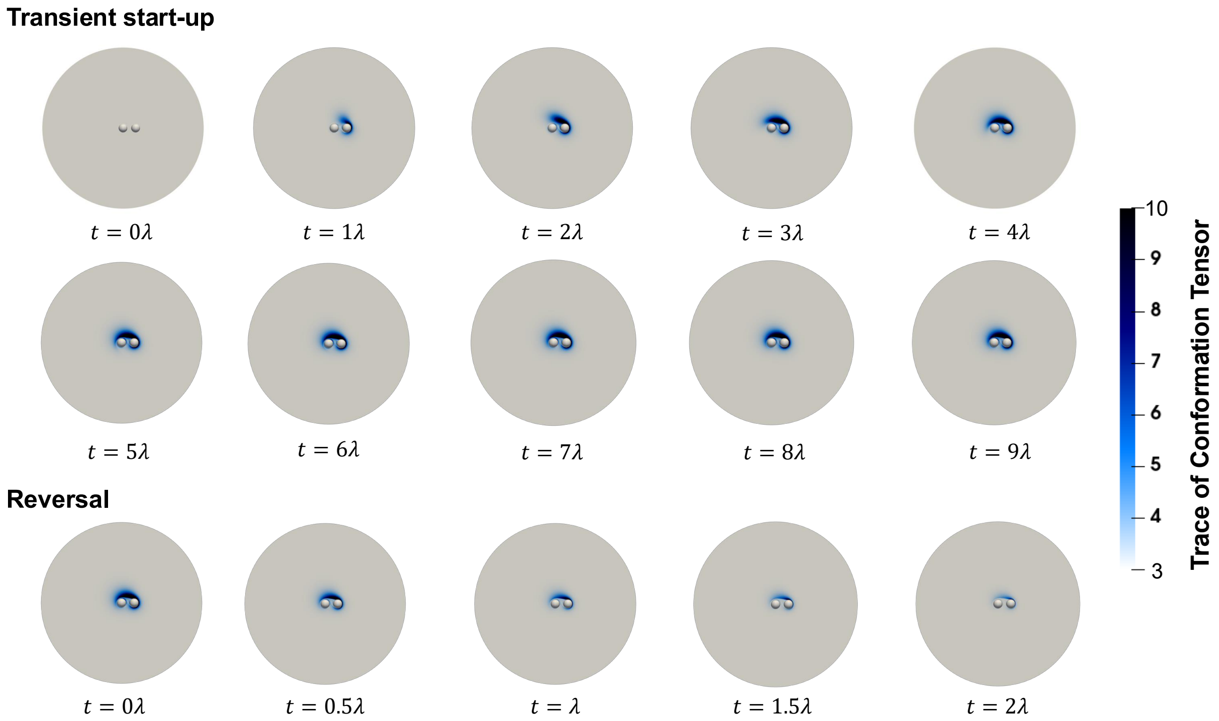


Figure S11: The trace of the conformation tensor in the plane of the 2 spheres, demonstrating the buildup of stress around the spheres during the transient start-up over multiple polymer relaxation times and the reversal trend for a separation of $r = 2.8a$ corresponding to $Wi = 3.5$ with $\beta = 0.1$.

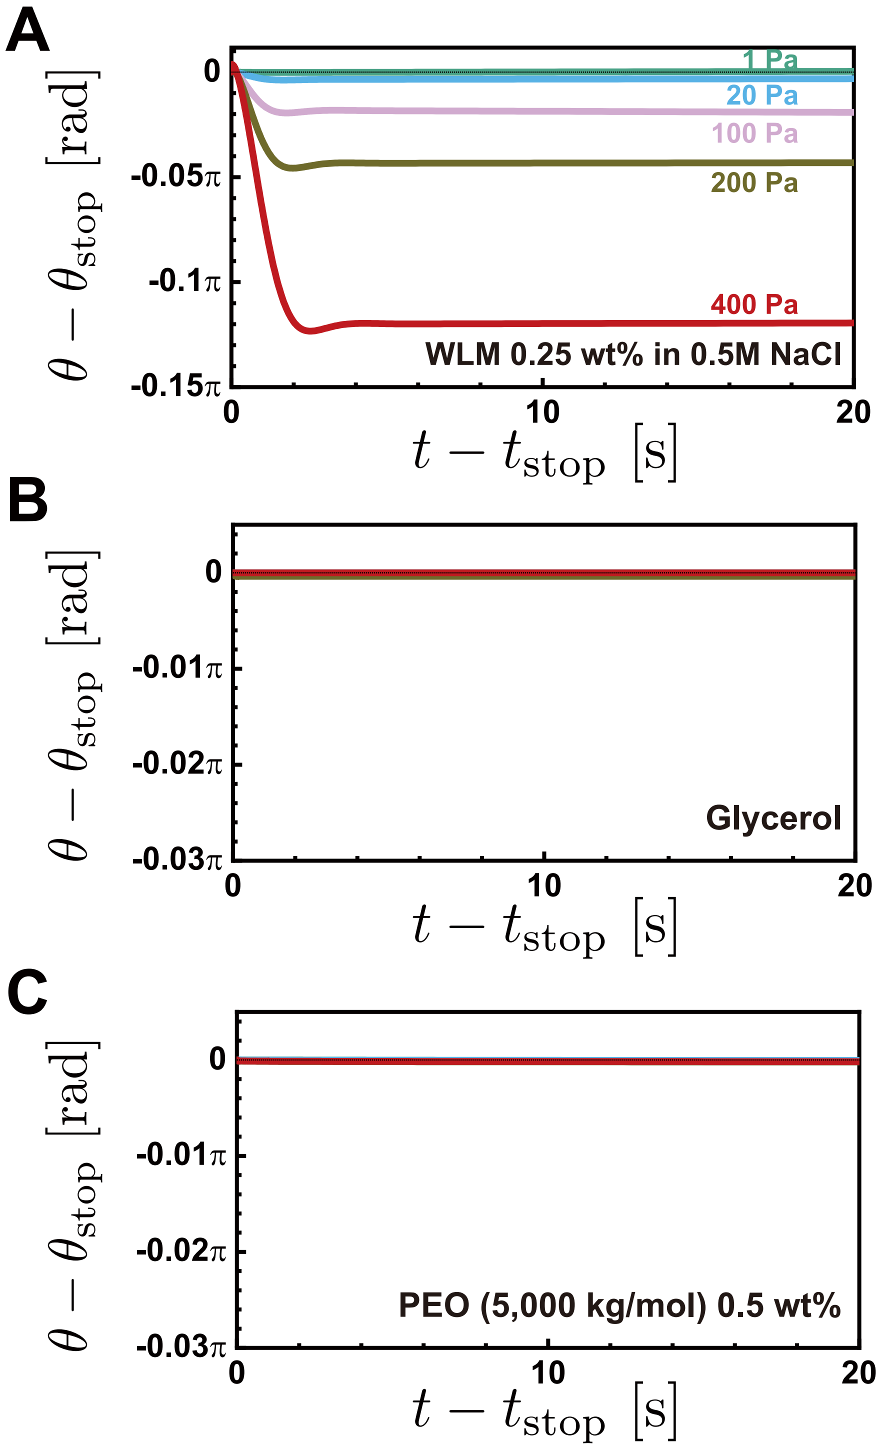


Figure S12: Macroscopic creep and recovery test of WLMs, glycerol and PEO solutions.To compare microscale and macroscale flow reversal, we performed creep-recovery measurements using a stress-controlled rheometer. A constant shear stress was applied for 20 s, followed by a 60 s recovery period under zero stress. (A) WLM solutions, (B) Glycerol, and (C) PEO solution.

were applied, consistent with the nonlinear elastic recovery hypothesis.

In contrast, glycerol and PEO samples exhibited no recovery with any sign of reverse deformation, regardless of the applied stress magnitude. These findings reinforce the conclusion that reversal is unique to systems with persistent elastic memory and arise only when sufficient network strain is imposed. Notably, the onset of reversal in the macrorheometer required higher stress than in our optical tweezer setup, likely due to differences in geometry, confinement, and the spatial averaging inherent to bulk rheological measurements.

# 4 Formulation of Stokesian dynamics for a suspension of colloids and bead-spring chains

In the following, we describe a modification of the Stokesian dynamics approach to simulate the (hydro)-dynamic interactions among few colloids and many polymers, represented using bead-spring chains. Interested readers are encouraged to see the work by Binous and Phillips [13].

At low Reynolds numbers, the solution to the equations of Stokes flow for the local velocity field may expressed as the following integral over the surface of the immersed particle centered at position $\boldsymbol{y}$,

$$u_i(\boldsymbol{x}) = \frac{1}{8\pi\eta_0} \oint_{S_p} J_{ij}(\boldsymbol{x}-\boldsymbol{y}) f_j(\boldsymbol{y}) \mathrm{d}S(\boldsymbol{y}). \tag{9}$$

We expand the surface force density into its first few multipole moments,

$$f_i(\boldsymbol{y}) = \frac{1}{4\pi a_s^2} F_i^H + \frac{3}{4\pi a_s^3} n_j(\boldsymbol{y}) C_{ij}^H + ..., \tag{10}$$

namely the hydrodynamic force

$$F_i^H = \oint_{S_p} f_i(\boldsymbol{y})\ \mathrm{d}S(\boldsymbol{y}), \tag{11}$$

and the first moment,

$$C_{ij}^H = \oint_{S_p} \left[ n_i(\boldsymbol{y}) f_j(\boldsymbol{y}) - \frac{1}{3}\delta_{ij}\Big( n_k(\boldsymbol{y}) f_k(\boldsymbol{y})\Big)\right]\ \mathrm{d}S(\boldsymbol{y}). \tag{12}$$

For a suspension containing multiple particles, the velocity field may be constructed from the linear superposition of Eqn. 9. After applying the multipole expansion, the approximate solution to the solvent velocity field arising from multiple immersed bodies is

$$\begin{aligned} u_i(\boldsymbol{x}) = \frac{1}{8\pi\eta_0} \sum_{\beta}^{N} \Bigg[ & \frac{1}{4\pi a_s^2} F_j^{H,(\beta)} \oint_{S_\beta} J_{ij}(\boldsymbol{x}-\boldsymbol{x}_\beta) \mathrm{d}S(\boldsymbol{y}) + \\ & \frac{3}{4\pi a_s^3} C_{jk}^{H,(\beta)} \oint_{S_\beta} n_k(\boldsymbol{x}_\beta) J_{ij}(\boldsymbol{x}-\boldsymbol{x}_\beta) \mathrm{d}S(\boldsymbol{x}_\beta) \Bigg]. \end{aligned} \tag{13}$$

We are interested in computing the fluid disturbances generated by a bidisperse mixture of few colloidal particles that are immersed in a suspension of bead-spring chains whose characteristic monomer sizes are smaller. As such, we expect that the hydrodynamic forces acting on the beads sufficiently represents their contribution to the local fluid disturbance. Larger colloidal particles require higher-order moments to incorporate the effects of finite size.

We modify Eqn. 13 by distinguishing between $N_c$ colloidal and $N_m$ monomeric particles based on their relative size. This is

$$
\begin{aligned}
u_i(\boldsymbol{x}) =& \frac{1}{8\pi\eta_0}\sum_{\alpha=1}^{N_c}\left[\frac{1}{4\pi a_c^2}F_j^{H,(\alpha)}\oint_{S_\alpha} J_{ij}(\boldsymbol{x}-\boldsymbol{x}_\alpha)\,\mathrm{d}S(\boldsymbol{x}_\alpha) + \right.\\
&\left.\qquad\qquad\frac{3}{4\pi a_c^3}C_{jk}^{H,(\alpha)}\oint_{S_\alpha} n_k(\boldsymbol{x}_\alpha)J_{ij}(\boldsymbol{x}-\boldsymbol{x}_\alpha)\,\mathrm{d}S(\boldsymbol{x}_\alpha)\right] \\
&+\frac{1}{8\pi\eta_0}\sum_{\beta=1}^{N_m}\frac{1}{4\pi a_m^2}F_j^{H,(\beta)}\oint_{S_\beta} J_{ij}(\boldsymbol{x}-\boldsymbol{x}_\beta)\,\mathrm{d}S(\boldsymbol{x}_\beta).
\end{aligned}
\tag{14}
$$

The objective of our simulation method is to determine the particle velocities and their hydrodynamic force moments simultaneously. Having now an expression for the solvent velocity field from the multipole moments, the particle kinematics may be determined from Faxén's relations,

$$
\begin{aligned}
U_i &= \frac{1}{4\pi a^2}\oint_{S_p} u_i(\boldsymbol{x})\mathrm{d}S(\boldsymbol{x}),\\
D_{ij} &= \frac{3}{4\pi a^3}\oint_{S_p} u_i(\boldsymbol{x})n_j(\boldsymbol{x})\mathrm{d}S(\boldsymbol{x}).
\end{aligned}
\tag{15}
$$

The symmetric and anti-symmetric components of $D_{ij}$ are the rotational velocity, $\boldsymbol{\Omega}_c$ and particle rate-of-strain, $\boldsymbol{E}_c$.

## 4.1 Grand mobility matrix

Substituting our approximation for the solvent velocity field into Faxén's relations, we obtain the linear relationship,

$$
\begin{bmatrix}\boldsymbol{U}_m\\ \begin{pmatrix}\mathcal{U}_c\\ \boldsymbol{E}_c\end{pmatrix}\end{bmatrix} = \begin{bmatrix}\mathcal{M}_{mm} & \mathcal{M}_{mc}\\ \mathcal{M}_{cm} & \mathcal{M}_{cc}\end{bmatrix}\begin{bmatrix}\boldsymbol{F}_m^H\\ \begin{pmatrix}\mathcal{F}_c^H\\ \boldsymbol{S}_c^H\end{pmatrix}\end{bmatrix},
\tag{16}
$$

or in its expanded form,

$$
\begin{bmatrix}\boldsymbol{U}_m\\ \boldsymbol{U}_c\\ \boldsymbol{\Omega}_c\\ \boldsymbol{E}_c\end{bmatrix} = \begin{bmatrix}\mathbf{M}_{mm}^{UF} & \mathbf{M}_{mc}^{UF} & \mathbf{M}_{mc}^{UL} & \mathbf{M}_{mc}^{US}\\ \mathbf{M}_{cm}^{UF} & \mathbf{M}_{cc}^{UF} & \mathbf{M}_{cc}^{UL} & \mathbf{M}_{cc}^{US}\\ \mathbf{M}_{cm}^{\Omega F} & \mathbf{M}_{cc}^{\Omega F} & \mathbf{M}_{cc}^{\Omega L} & \mathbf{M}_{cc}^{\Omega S}\\ \mathbf{M}_{cm}^{EF} & \mathbf{M}_{cc}^{EF} & \mathbf{M}_{cc}^{EL} & \mathbf{M}_{cc}^{ES}\end{bmatrix}\begin{bmatrix}\boldsymbol{F}_m^H\\ \boldsymbol{F}_c^H\\ \boldsymbol{L}_c^H\\ \boldsymbol{S}_c^H\end{bmatrix}.
\tag{17}
$$

The subscripts "$m$" and "$c$" correspond to monomers and colloids, respectively. Dual subscripts in the mobility matrices indicate pair hydrodynamic interactions between monomers only, monomers and colloids, and colloids only. We distinguish monomers and colloids based on their respective sizes, whose ratio appears in the mobility matrices with the "$mc$" and "$cm$" subscripts. In our notation, $\mathcal{M}_{mm} = \mathbf{M}_{mm}^{UF}$, $\mathcal{U}_c = (\boldsymbol{U}_c \quad \boldsymbol{\Omega}_c)^T$, and $\mathcal{F}_c^H = \left(\boldsymbol{F}_c^H \quad \boldsymbol{T}_c^H\right)^T$ Analytical expressions for the pair mobilities are tabulated [14].

## 4.2 Force and torque balances

To close the problem, we couple the mobility relation to the force and torque balances. Ignoring thermal fluctuations, these are

$$
\boldsymbol{F}_m^H + \boldsymbol{F}_{mm}^P + \boldsymbol{F}_{mc}^P + \boldsymbol{F}_m^{\mathrm{ext}} = \mathbf{0},
\tag{18}
$$

$$\boldsymbol{F}_c^H + \boldsymbol{F}_{cc}^P + \boldsymbol{F}_{cm}^P + \boldsymbol{F}_c^{\text{ext}} = \mathbf{0}, \tag{19}$$

$$\boldsymbol{L}_c^H + \boldsymbol{L}_c^{\text{ext}} = \mathbf{0}. \tag{20}$$

$\boldsymbol{F}^P$ denotes pair interactions that are driven by a potential gradient, and $\boldsymbol{F}^{\text{ext}}$ describes externally applied fields (e.g., harmonic traps). Dual subscripts represent the interactions between the two particle types. For example, $\boldsymbol{F}_{mm}^P$ includes the force-extension law that describes the bonds between monomer pairs. Here, we use Hooke's law. Then, the bond force on a given bead, $\alpha$, is found by summing over its bonded pairs, $\boldsymbol{F}_{mm}^{(\alpha)} = -\sum_{\beta \in \{\text{bonds}(\alpha)\}} k^{(\alpha)(\beta)}(r^{(\alpha)(\beta)} - r_0^{(\alpha)(\beta)})\hat{\boldsymbol{r}}^{(\alpha)(\beta)}$. We take the stiffness, $k^{(\alpha)(\beta)}$, and the resting bond length, $r_0^{(\alpha)(\beta)}$, to be constant. We specify motion on the colloidal spheres by a moving trapping potential with a predetermined trajectory to mimic, $\boldsymbol{F}_c^{\text{ext}} = -k_{\text{trap}}(\boldsymbol{x}_c(t) - \boldsymbol{x}_{\text{trap}}(t))$. We allow overlaps between the monomeric beads, and we prevent overlaps between them and the larger colloidal particles using the procedure by Melrose and Heyes [15]. Lastly, $\boldsymbol{L}_c^{\text{ext}} = \mathbf{0}$, so that the colloids rotate freely.

### 4.3 Saddle point formulation

The induced flows generated by the monomeric beads and colloidal particle must satisfy the over-damped force and torque balances. We handle this coupling using a saddle point system [16]. Writing the mobility relation, Eqn. 17, as $\mathcal{U} = \mathcal{M} \cdot \mathcal{F}$, we separate the desired monomeric and colloidal velocities,

$$\mathcal{M} \cdot \mathcal{F} + \mathcal{B} \cdot \begin{pmatrix} \boldsymbol{U}_m \\ \boldsymbol{U}_c \\ \boldsymbol{\Omega}_c \end{pmatrix} = \begin{pmatrix} \mathbf{0} \\ \mathbf{0} \\ \mathbf{0} \\ \boldsymbol{E}_c \end{pmatrix}. \tag{21}$$

We have used the non-square projection matrix, $\mathcal{B}$, defined such that $-\mathcal{B} \cdot (\boldsymbol{U}_m \;\; \boldsymbol{U}_c \;\; \boldsymbol{\Omega}_c)^T = (\boldsymbol{U}_m \;\; \boldsymbol{U}_c \;\; \boldsymbol{\Omega}_c \;\; \mathbf{0})^T$. The transpose of this operator projects the generalized vector of force moments onto a smaller subspace that contains the far-field hydrodynamic forces and torques. Together, the mobility and force relations form the saddle point system,

$$\begin{bmatrix} \mathcal{M} & \mathcal{B} \\ \mathcal{B}^T & \mathbf{0} \end{bmatrix} \begin{bmatrix} \mathcal{F} \\ \mathbb{U} \end{bmatrix} = \begin{bmatrix} \begin{pmatrix} \mathbf{0} \\ \boldsymbol{E}_c \end{pmatrix} \\ -\mathbb{F}^C \end{bmatrix}, \tag{22}$$

generically denoting the unknown kinematic quantities and their net forces (and torques) through $\mathbb{U}$ and $\mathbb{F}^C$, respectively. In the absence of externally-imposed straining flows, rigidity of the immersed particles reuqires that $\boldsymbol{E}_c = \mathbf{0}$.

At each timestep, we construct the grand mobility matrix from the particle positions. We retain monomer-colloid and colloid-colloid hydrodynamic interactions, while ignoring the pair interactions between the monomeric beads themselves. That is, $\mathcal{M}_{mm} = (a_m/a_c)\mathbf{I}$. As the total number of pairs among all particles (colloidal and monomeric) is dominated by those between monomeric beads, ignoring their pair hydrodynamic coupling significantly reduces computation times.

## 5 Supplemental Movies

**Movie S1.** Time-lapse videos of optical laser tweezer experiments in Newtonian and viscoelastic fluids. The viscoelastic medium is a wormlike micellar solution composed of 0.25 wt% in water. In

both cases, the center-to-center distance between the colloidal particles is fixed at 7 µm, and the imposed velocity of the moving colloid is maintained at 60 µm/s.

**Movie S2.** Delayed angular response in a viscoelastic medium. This video compares the rotation of a trapped probe particle in water and in a wormlike micellar solution (0.125 wt% in 0.5 M NaCl) when a neighboring colloid is driven along a circular trajectory at 60 µm/s. The particles are separated by a center-to-center distance of 7 µm. In the WLM solution, the initial angular displacement of the probe is smaller than in water. The scale bar represents 5 µm.

**Movie S3.** Reversal in angular displacement after stopping the driven particle. This video shows the rotational response of a fixed probe particle in a wormlike micellar solution after the driving colloid is stopped following several circular revolutions. The particles are separated by a center-to-center distance of 7 µm. After cessation of motion, reversal flows emerge in the viscoelastic medium, driving the angular displacement $\theta(t)$ of the probe in the opposite direction. The scale bar represents 5 µm.

**Movie S4.**Sample Stokesian dynamics simulation of colloidal particles in a bath of bead-spring chains. This movie shows two colloidal particles of size $a_c$ (gray) immersed in a viscoelastic medium represented using bead-spring trimers (yellow lines indicate bond connections). The monomer bead size is $a_m = 0.1a_c$ (pink). The driven particle completes two orbits about a stationary probe, maintaining the center-to-center distance $r = 2.8a_c$. The motion of the driven particle distorts the microstructure of the polymeric bath. After cessation, the hydrodynamic forces stored in stretched bonds relax, further producing disturbance flows that induce reversal in the angular displacement of the stationary probe (see main text for more details).

**Movie S5.**Stress generation and relaxation in bead-spring simulations. This movie visualizes the evolution of monomeric bead density and polymer stress obtained from Stokesian dynamics simulations. As the driven colloidal particle orbits the stationary probe, monomeric beads accumulate at the front and are depleted in the wake, producing a non-uniform monomer density field, $\langle n^m \rangle(\boldsymbol{x}, t)$. We measure the magnitude of the hydrodynamic torque at each monomeric bead, $\langle |\boldsymbol{X}^m \wedge \boldsymbol{F}^{H,m}| \rangle(\boldsymbol{x}, t)$. Chains are stretched and aligned near the moving particle, generating elastic stresses that persist after motion ceases. Normal stress also develops, $-\frac{1}{2}\langle \boldsymbol{X}^m \cdot \boldsymbol{F}^{H,m} \rangle(\boldsymbol{x}, t)$. Positive stress acts on the outward faces of the colloidal particles and opposing stress persists in their interfacial gap. See main text for further discussion surrounding these quantities.

**Movie S6.**Attraction between colloids after winding in a WLM solution. This video shows two colloidal particles immersed in a WLM solution, initially held at a center-to-center distance of 7.0 µm under strong trapping. One particle is driven along a circular trajectory around the stationary probe for 10 windings, and the trap stiffness is then greatly reduced. Following this change, the particles move toward each other due to stress-induced attraction in the viscoelastic medium. The scale bar represents 10 µm.

**Movie S7.**Hydrodynamic attraction between colloids following straining a polymeric medium. This movie presents a Stokesian dynamics simulation of two colloidal particles embedded in a bath of bead-spring chains. The driven particle completes one orbit around a stationary probe with fixed separation distance, after which the trapping strength is reduced. The relaxation of hydrodynamic forces stored in bonds induces an attraction between the two particles.

**Movie S8.**Rotational motion of colloidal particles in a finite hexagonal array during oscillatory shear in a viscoelastic fluid. Seven colloids are initially arranged in a finite hexagonal lattice in wormlike micellar solution. We apply small-amplitude oscillatory strain to the structure and measure the rotational velocity of the central sphere as a function of packing fraction and oscillation frequency.

# References


[1] ME Cates. Reptation of living polymers: dynamics of entangled polymers in the presence of reversible chain-scission reactions. *Macromolecules*, 20(9):2289–2296, 1987.

[2] R Granek and ME Cates. Stress relaxation in living polymers: Results from a poisson renewal model. *Journal of Chemical Physics*, 96(6):4758–4767, 1992.

[3] Ronald G Larson. The lengths of thread-like micelles inferred from rheology. *Journal of Rheology*, 56(6):1363–1374, 2012.

[4] Danila Gaudino, Rossana Pasquino, and Nino Grizzuti. Adding salt to a surfactant solution: Linear rheological response of the resulting morphologies. *Journal of Rheology*, 59(6):1363–1375, 2015.

[5] C Oelschlaeger, M Schopferer, Frank Scheffold, and N Willenbacher. Linear-to-branched micelles transition: A rheometry and diffusing wave spectroscopy (dws) study. *Langmuir*, 25(2):716–723, 2009.

[6] Vesselin N Paunov. Novel method for determining the three-phase contact angle of colloid particles adsorbed at air- water and oil- water interfaces. *Langmuir*, 19(19):7970–7976, 2003.

[7] William H Press, Saul A Teukolsky, William T Vetterling, and Brian P Flannery. Numerical recipes in fortran 77. *The art of scientific computing*, 1, 1992.

[8] Mengfei Yang, Sreenath Krishnan, and Eric SG Shaqfeh. Numerical simulations of the rheology of suspensions of rigid spheres at low volume fraction in a viscoelastic fluid under shear. *Journal of Non-Newtonian Fluid Mechanics*, 233:181–197, 2016.

[9] David Richter, Gianluca Iaccarino, and Eric SG Shaqfeh. Simulations of three-dimensional viscoelastic flows past a circular cylinder at moderate reynolds numbers. *Journal of Fluid Mechanics*, 651:415–442, 2010.

[10] Jonas Einarsson, Mengfei Yang, and Eric SG Shaqfeh. Einstein viscosity with fluid elasticity. *Physical Review Fluids*, 3(1):013301, 2018.

[11] Anni Zhang, William L Murch, Jonas Einarsson, and Eric SG Shaqfeh. Lift and drag force on a spherical particle in a viscoelastic shear flow. *Journal of Non-Newtonian Fluid Mechanics*, 280:104279, 2020.

[12] Dae Yeon Kim, Sachit G Nagella, Kyu Hwan Choi, and Sho C Takatori. Direct experimental measurement of many-body hydrodynamic interactions with optical tweezers. *Physical Review Fluids*, 10(6):064301, 2025.

[13] Housam Binous and Ronald J Phillips. Dynamic simulation of one and two particles sedimenting in viscoelastic suspensions of FENE dumbbells. *Journal of Non-Newtonian Fluid Mechanics*, 83(1-2):93–130, June 1999.

[14] Sangtae Kim and Seppo J Karrila. *Microhydrodynamics*. Butterworth-Heinemann Series in Chemical Engineering. Butterworth-Heinemann, Oxford, England, February 1991.

[15] D M Heyes and J R Melrose. Brownian dynamics simulations of model hard-sphere suspensions. *Journal of Non-Newtonian Fluid Mechanics*, 46(1):1–28, January 1993.

[16] Andrew M Fiore and James W Swan. Fast stokesian dynamics. *Journal of Fluid Mechanics*, 878:544–597, November 2019.
